# Supplementary material for: From Pixels to Objects: A Hierarchical Approach for Part and Object Segmentation Using Local and Global Aggregation
Source: arXiv:2409.01353 source file (2024-09-02)
Supplement: Supplementary file 1 [file A_appendix.tex]

\section{Appendix}
